# Supplementary material for: All That's 'Human' Is Not Gold: Evaluating Human Evaluation of Generated Text
Source: arXiv:2107.00061 source file (2021-07-07)
Supplement: Supplementary file 1 [file 8_supplementary.tex]

\clearpage \newpage

\section{Supplementary Material}
This document contains the model priming texts and evaluator training materials for ``All That's `Human' Is Not Gold:  Evaluating Human Evaluation of Generated Text.''

\subsection{Priming Texts}\label{sup:exemplars}
When generating the text passages, we conditioned the text on three in-domain, human-authored texts. The exact passages we used for each domain are in Tables \ref{tab:story_exemplars}--\ref{tab:recipe_exemplars}.

\begin{table*}[h]
\small
\begin{tabular}{p{\linewidth}}
\toprule
Once upon a time magic was an art. The great magicians of the time would take on apprentices who would train for a decade or more, slaving under their tutelage for the hope of one day being the next great magician. They were free from the bonds of apprenticeship only once they had made the perfect magic circle. Only then could they harness the power of the mages and go off on their own. But times changed, magicians were persecuted, and few longed to toil away for the long years of study necessary. In the course of a century, magic became extinct. \\
\midrule
\begin{tabular}[c]{@{}p{\linewidth}@{}}Once upon a time, there lived an old woman. She was as you'd expect an old woman to be in most respects, brittle and stooped as though whatever foundation still held her old bones up might break at any minute and cause the whole abode to come tumbling down. Her eyes were glazed like a bakers treats - what they'd come to call cataracts in years to come. Her joints were all swollen, such that her fingers were like poorly balanced, chubby spiders from a children's tale. But not all was as one thinks an old woman should be.\\ \\ She was wise beyond sight.\end{tabular} \\
\midrule
\begin{tabular}[c]{@{}p{\linewidth}@{}}Once upon a time, there lived a boy who was a close friend to the princess of a rival town.\\ \\ They, despite the many warnings made by their fathers, were close to one another, often seen sneaking pieces of raided pies from the marketplace vendors and chasing each other in the meadows that rested between the two towns.\\ \\ For many years, the townspeople tolerated their friendship, many secretly hoping that it would lead to a truce between each other.\\ \\ However, on the boy's fifteenth birthday, the uneasy peace between the rivaling factions was shattered as rumors of the princess being kidnapped spread and sparked an almost palatable bloodlust in the girl's people.\end{tabular} \\
\bottomrule
\end{tabular}
\caption{The three passages used to condition the generated story text.}\label{tab:story_exemplars}
\end{table*}

\begin{table*}[h]
\small
\begin{tabular}{p{\linewidth}}
\toprule
\begin{tabular}[c]{@{}p{\linewidth}@{}}Headline: New Jersey Devils' affiliate moves from Binghamton to Newark for 2021 AHL season\\ Article: Come anticipated Feb. 5 commencement of the American Hockey League’s abbreviated season, the Binghamton Devils will call Newark, New Jersey, home. AHL President and Chief Executive Officer Scott Howson disclosed the 2020-21 season will include 28 teams operating in five divisions. Four have been granted provisional relocation for the 2020-21 season: The B-Devils in Newark; the Ontario Reign in El Segundo, California; the Providence Bruins in Marlborough, Massachusetts; and the San Diego Gulls in Irvine, California. ``We've gone back and forth with (parent club) New Jersey about how to get through this COVID situation and we've looked at all the expenses, and — they have the final decision on all this stuff,'' said Tom Mitchell, B-Devils Executive Vice President of Operations.\end{tabular} \\
\midrule
\begin{tabular}[c]{@{}p{\linewidth}@{}}Headline: Connecticut’s Beardsley Zoo Welcomes New River Otter Following Renovation of Habitat\\ Article: Connecticut’s Beardsley Zoo is the new home for Tahu, a one-year-old female North American river otter newly arrived from the Woodland Park Zoo in Seattle, Wash. After the Zoo’s last river otter passed away in 2019 from advanced age, the Zoo engaged in long-planned improvements to the otter habitat. With renovations complete, Tahu has joined the Zoo family and will be joined by a male companion in the future. As a species, river otters have suffered from habitat loss, water pollution, and fur trapping. Their numbers are on the rise due to reintroduction programs in parts of the U.S., better water quality, and protection of their habitats. Zoo Director Gregg Dancho said, ``Our river otters have always been some of the most popular animals who make their home here at the Zoo, for their playful nature and intelligence as well as their role as an iconic North American animal.\end{tabular} \\
\midrule
\begin{tabular}[c]{@{}p{\linewidth}@{}}Headline: Johnson City eyesore to get a makeover: This is what you may see from Rt. 17\\ Article: Construction to transform the long-vacant Endicott Johnson Victory building, often described as Broome County's "biggest eyesore," into 108 market-rate apartments plus commercial space is expected to get underway in the fall of 2021. The anticipated \$30-million project and its targeted completion date of 2023 was announced Monday by Paulus Development, the Syracuse-based firm that renovated the former Ansco factory on Binghamton's West Side into a multi-unit apartment building. The developers acquired the Johnson City parcel at 59 Lester Ave. in March. Matthew Paulus, president of Paulus Development, said the apartments will contain modern amenities and enclosed parking, along with 7,500 square feet of retail space. It's anticipated renters would include young professionals and empty-nesters among others. "Where there is a lot of additional opportunity are people that will be coming in for private sector or public sector jobs.\end{tabular} \\
\bottomrule
\end{tabular}
\caption{The three passages used to condition the generated news text.}\label{tab:news_exemplars}
\end{table*}

\begin{table*}[h]
\small
\begin{tabular}{p{\linewidth}}
\toprule
\begin{tabular}[c]{@{}p{\linewidth}@{}} Title: All-Natural Strawberry Sauce\\ Ingredients:\\ 2 cups fresh strawberries\\ 13 cup good quality honey\\ 1 vanilla bean, split open, seeds removed and included\\ 1 12 tablespoons good balsamic vinegar\\ Recipe:\\ Roughly chop the strawberries and toss the pieces into a 2 quart saucepan.\\ Add honey, vanilla bean, and seeds and bring to a boil.\\ You may have to add 1/4 C of water, depending on how juicy your strawberries are.\\ Cook the mixture until the strawberries are tender and cooked, about 10 minutes.\\ As long as you leave the mixture on medium heat, you can walk away from pot.\\ Just make sure the pot has enough moisture so the sauce wont burn (you can add more water if necessary).\\ When the strawberries are cooked and the sauce thickens to a syrup-like consistency, add the balsamic vinegar and continue to cook for a few minutes longer to thicken again.\end{tabular} \\
\midrule
\begin{tabular}[c]{@{}p{\linewidth}@{}} Title: Crispy Potato Cake\\ Ingredients:\\ 4 large russet or Idaho potatoes (about 2 pounds), peeled\\ 1 1/4 teaspoons salt\\ 18 teaspoon pepper\\ 1/4 cup vegetable oil, plus more as needed\\ Recipe:\\ Using a mandolin or food processor, julienne the potatoes.\\ Toss with salt and pepper.\\ In a 12-inch skillet, heat the oil over high heat until very hot but not smoking.\\ Add the potatoes and press with the back of a spatula to form an even layer.\\ Lower the heat to medium and cook until the bottom is golden brown, 10 to 20 minutes, shaking the pan frequently so the potatoes don't stick and adding oil as needed.\\ Flip the potato cake, add more oil if necessary and cook until the other side is golden brown.\\ Cool the cake briefly on a wire rack and cut into 6 wedges.\end{tabular} \\
\midrule
\begin{tabular}[c]{@{}p{\linewidth}@{}} Title: Sesame-Ginger Salmon With Braised Bok Choy\\ Ingredients:\\ 1 1/2 pounds bok choy\\ 2 teaspoons minced garlic\\ 4 teaspoons salad oil\\ 3/4 cup fat-skimmed chicken broth\\ 1 1/2 pounds boned salmon fillet with skin (maximum 1 in. thick)\\ 4 teaspoons sesame seed\\ 1 1/2 teaspoons ground ginger\\ Recipe:\\ Rinse bok choy; trim off and discard tough stem ends and any bruised parts. Cut the leafy tops crosswise into 2-inch strips; cut the stems crosswise into 1-inch pieces.\\ In a 10- to 12-inch frying pan over high heat, stir garlic in 2 teaspoons oil until sizzling, 1 to 2 minutes. Add bok choy and broth, cover, and cook until thickest stems are just tender when pierced, 4 to 5 minutes; keep warm.\\ Meanwhile, rinse salmon, pat dry, and cut into 4 equal pieces. Mix sesame seed with ginger, and rub fish evenly with mixture. Pour remaining 2 teaspoons oil into a 10- to 12-inch frying pan over high heat.\end{tabular} \\
\bottomrule
\end{tabular}
\caption{The three passages used to condition the generated recipe text.}\label{tab:recipe_exemplars}
\end{table*}

\begin{table*}[]
\small
\begin{tabular}{p{.5\linewidth}p{.5\linewidth}}
\toprule
GPT3 & Human \\
\midrule
\begin{tabular}[c]{@{}p{\linewidth}@{}}\textbf{*Once upon a time}, there was a man in a place that was not a place at all.\\ \\ He didn't know anything of a place or a time or who he was or what he was doing there. There was just him and the silence.\\ \\ He sat there for a long time, not knowing what he was doing there. He thought, thought and thought, but he didn't know what to think. There was just him and the silence. He tried to speak, but no sound came from his mouth. He tried to move, but his body would not move. He sat there, but he didn't know for how long he was there.\end{tabular} & \begin{tabular}[c]{@{}p{\linewidth}@{}}\textbf{Once upon a time}, there lived a little girl who ran around the village wearing a little red riding hood. Don't ask me what a riding hood is because I don't even know. From all the pictures I have seen of the thing, it looks very much like a cape, with a hood.\\ \\ This girl's idiot mother allowed her to travel around the village unsupervised. Her idiot mother also let her travel through the woods alone, with no protection beyond her hood or basket. Not a very smart parent, if you ask me. This girl can't have been older than ten or eleven.\end{tabular} \\
\midrule
\multicolumn{2}{p{\linewidth}}{\textbf{Comment:} Note how the {[}machine-authored{]} story is repetitive and doesn't seem to go anywhere.} \\
\midrule
\begin{tabular}[c]{@{}p{\linewidth}@{}}\textbf{Once upon a time}, there was a girl who was born a princess. Her birth was not unexpected; her father had long since wanted a daughter, and her mother had long since been unable to give him one. So it was that when, after years of childless marriage, a daughter was born, they rejoiced.\\ \\ The girl was raised in the lap of luxury, and as she grew, she came to expect that the world would be at her beck and call. The girl who had once been pampered and coddled was now pampered and coddled, and grew to be quite the vain, spoiled brat.\end{tabular} & \begin{tabular}[c]{@{}p{\linewidth}@{}}\textbf{*Once upon a time}, in a faraway land, a princess scowled at the newspaper. Another of her friends had been kidnapped. Another! that made six this month. She tore the thing neatly in two and almost threw it at her handmaiden, declaring, ``this has to stop. I mean, isn't life difficult enough for princesses without the constant threat of kidnap hanging over our heads?''\\ \\ The maid raised a delicate eyebrow, her thoughts turning to her own difficulties, so far removed from those of her employer, ``highness, I don't think there's anything to be done about it ...'' she complained.\\ \\ This was met with a disparaging look from Princess Ellionora, who rose to her feet, dislodging one of the flowers in her hair with a sudden head movement.\end{tabular}  \\
\midrule
\multicolumn{2}{p{\linewidth}}{\textbf{Comment: }Note that though there are some capitalization errors, the {[}human-authored{]} story is original and engaging.} \\
\midrule
\begin{tabular}[c]{@{}p{\linewidth}@{}}\textbf{*Once upon a time}, there lived a girl who was the daughter of the greatest wizard of her time.\\ \\ She was the daughter of the great wizard, yet she was not a very good magician.\\ \\ Her father instructed her to practice her magic every day. He told her to polish off the dust of the books in his library, clean the dishes in the kitchen, and sweep the front of the house.\\ \\ She did not enjoy her chores.\\ \\ She wanted to go with the other girls in the village and play. But she had to do her chores.\end{tabular} & \begin{tabular}[c]{@{}p{\linewidth}@{}}\textbf{Once upon a time}, there was a young man named Neil. Neil's family was made up of warriors on his mother's side, and poets on his father's side.\\ \\ His parents were certain that Neil would take up one or the other profession. But Neil had no interest in bloodshed, and suffered from a terribly tied tongue. And from the time he could read, to to the time when he was ten years old, Neil felt alone in his own family, a self-imposed outcast.\\ \\ However, one day, Neil saw something that changed his perspective on life. A visiting dignitary had come to the tribe to seek an alliance with them.\end{tabular} \\
\midrule
\multicolumn{2}{p{\linewidth}}{\textbf{Comment:} Note that there seem to be some inconsistencies {[}in the machine-generated story{]}; first it says the father orders her to practice magic, then it says he orders her to do chores.} \\
\bottomrule
\end{tabular}
\caption{The training materials used in the story domain for the Comparison trainings. The passages marked with * were shown in the Example training, along with the comments with the bracketed text removed.}
\label{tab:news_training}
\label{tab:story_training}
\end{table*}

\begin{table*}[]
\small
\begin{tabular}{p{.5\linewidth}p{.5\linewidth}}
\toprule
GPT3 & Human \\
\midrule
\begin{tabular}[c]{@{}p{\linewidth}@{}}\textbf{*Headline: Twitter reacts to former South Dakota QB Chris Streveler playing for Arizona Cardinals}\\ \textbf{Article: Former University of South Dakota quarterback Chris Streveler replaced Arizona Cardinals QB Kyler Murray, and South Dakotans are loving it.} Streveler, who is from Mitchell, completed two of his three passes for 44 yards, including a pass to Larry Fitzgerald for a touchdown. "I just had to get an opportunity, and I got it, and I'm grateful for that," Streveler said. "I'm just trying to take advantage of it." Streveler was the first player in University of South Dakota history to throw for more than 9,000 yards.\\ \\ Headline: RHI program to help offset carbon emissions from I-90 bridge rebuild\\ Article: The \$7 billion Gateway Project to replace the aging, often-congested, and increasingly dangerous Hudson River crossings between New York and New Jersey has received a major boost by a new agreement to offset carbon emissions from the project.\end{tabular} & \begin{tabular}[c]{@{}p{\linewidth}@{}}\textbf{Headline: Twitter reacts to former South Dakota QB Chris Streveler playing for Arizona Cardinals}\\ \textbf{Article: Former University of South Dakota quarterback Chris Streveler replaced Arizona Cardinals QB Kyler Murray, and South Dakotans are loving it.} It became Chris Streveler time for the Cardinals early in the first quarter when Murray went down with a right ankle injury. Streveler completed his first NFL pass to Trent Sherfield and then tossed a pass to Jonathan Ward, who ran past several Los Angeles Rams' defenders for a touchdown — the first of Streveler's professional career. The touchdown catch was Ward's first touch of his career. Streveler did throw a pick-six just before halftime, giving the Rams a 12-7 lead. The 6-foot-1 216-pound Streveler played sparingly earlier this season, but only for a few short run plays. With a win in Sunday's game, the Cardinals would make the playoffs.\end{tabular} \\
\midrule
\multicolumn{2}{p{\linewidth}}{\textbf{Comment:} Note that the {[}machine-generated{]} article doesn't mention many of the things brought up in the title or the first line of the article, and note how the article turns into a new headline.} \\
\midrule
\begin{tabular}[c]{@{}p{\linewidth}@{}}\textbf{Headline: One dead in Gering fire}\\ \textbf{Article: Authorities have confirmed firefighters found one person deceased in a Gering fire this afternoon (Thursday).} Gering Fire Chief John Scharfenberg says crews were dispatched to a one-story commercial building at the corner of Lincoln and 13th Street shortly before 2:30 Thursday afternoon. When crews arrived, they found heavy fire coming from the structure. They say one person was in the building at the time, but was able to get out safely. The Gering Fire Department received mutual aid from the Gering-Kimi Fire Protection District, Scottsbluff Fire Department, Scottsbluff Ambulance, Scottsbluff Police Department, and the Scottsbluff Housing Authority. Crews were able to put the fire out by around 5:30 Thursday evening.\end{tabular} & \begin{tabular}[c]{@{}p{\linewidth}@{}}\textbf{*Headline: One dead in Gering fire}\\ \textbf{Article: Authorities have confirmed firefighters found one person deceased in a Gering fire this afternoon (Thursday).} Firefighters responded to a home in the 1200 block of R Street at about 2:30 p.m. The Gering Fire Department and Scottsbluff Fire Department responded to the fire. Gering Fire Department Chief Nathan Flowers said his department received a call that smoke was emanating the structure on R street, near Lincoln Elementary School. When firefighters arrived on the scene, Flower said smoke was pouring from the windows of the small house. He said it took about half an hour to subdue the blaze and, upon entry, firefighters discovered the body. ``There was one occupant that lived in the structure. We did find the occupant deceased in the structure.\end{tabular} \\
\midrule
\multicolumn{2}{p{\linewidth}}{\textbf{Comment:} Note how {[}in the human-authored article,{]} Nathan Flowers is introduced by his full title before shortening his name and giving his quote.} \\
\midrule
\begin{tabular}[c]{@{}p{\linewidth}@{}}\textbf{*Headline: Fisher Scones parent company fined for overworking teenage employees}\\ \textbf{Article: Washington State Department of Labor and Industries found more than 1,500 instances of violations including missing meal breaks, working during school hours and more.} Fisher Scones, Inc., the parent company of Fisher Scones Bakery \& Café, has agreed to pay \$36,000 in fines for overworking teenage employees. The Washington State Department of Labor and Industries (L\&I) found more than 1,500 instances of violations including missing meal breaks, working during school hours and more. The company has agreed to pay \$36,000 in fines and will also implement an internal training program to prevent future violations. ``Fisher Scones has been a leading business in this region for many years,'' said David LaBarre, director of L\&I’s Spokane office. ``Despite their success, we found hundreds of violations over a three-year period. That’s simply unacceptable.''\end{tabular} & \begin{tabular}[c]{@{}p{\linewidth}@{}}\textbf{Headline: Fisher Scones parent company fined for overworking teenage employees}\\ \textbf{Article: Washington State Department of Labor and Industries found more than 1,500 instances of violations including missing meal breaks, working during school hours and more.} The parent company of fair staple and fan favorite Fisher Scones has been fined for more than 1,500 instances of overworking teenage employees beyond hours allowed under Washington state law, according to a Dec. 16 announcement from the Washington State Department of Labor \& Industries. Fisher Scones, under parent company Conifer Foods based in Woodinville, specializes in buttery, raspberry jam-filled scones at the Washington State Fair in Puyallup, Evergreen State Fair in Monroe and a variety of roaming food truck locations. The company started in 1977. The citation includes a \$45,100 fine, which Conifer Foods has until Dec. 23 to appeal, and includes the most work-hour violations involving minors that the state’s L\&I department has ever found, according to a release.\end{tabular} \\
\midrule
\multicolumn{2}{p{\linewidth}}{\textbf{Comment:} Note how the first line {[}of the machine-authored article{]} is repeated later on, almost verbatim.} \\
\bottomrule
\end{tabular}
\caption{The training materials used in the news domain for the Comparison trainings. The passages marked with * were shown in the Example training, along with the comments with the bracketed text removed.}
\label{tab:news_training}
\end{table*}

\begin{table*}[]
\tiny
\begin{tabular}{p{.5\linewidth}p{.5\linewidth}}
\toprule
{\small GPT3} & {\small Human} \\
\midrule
\begin{tabular}[c]{@{}p{\linewidth}@{}}\textbf{*Title: Ricotta Panna Cotta With Basil Balsamic Strawberries}\\ \textbf{  Ingredients:}\\ \textbf{ Ricotta Panna Cotta}\\ \textbf{ 2 1/2 teaspoons unflavored gelatin}\\ \textbf{ 5 tablespoons water}\\ \textbf{ 2 cups whipping cream}\\ \textbf{ 2/3 cup icing sugar}\\ \textbf{ 1 cup ricotta cheese}\\ \textbf{ 1/2 vanilla bean, slit lengthwise}\\ \textbf{ Basil Balsamic Strawberries}\\ \textbf{ 1 lb strawberry}\\ \textbf{ 1/3 cup orange juice}\\ \textbf{ 2 tablespoons balsamic vinegar}\\ \textbf{ 1/2 teaspoon cracked black pepper}\\ \textbf{ 6 large basil leaves, shredded}\\ \textbf{ Recipe:}\\ Pour water into a small bowl and sprinkle with gelatin, set aside.\\ 2. In a saucepan, heat cream, sugar and vanilla bean until it starts to boil, set aside.\\ 3. In a medium sized bowl, whisk together the ricotta cheese and the vanilla bean scrapings.\\ 4. Pour the warm cream mixture into the ricotta mixture and whisk until well combined.\\ 5. Pour into 4 small serving dishes.\\ 6. Pour the gelatin mixture over the panna cottas. Set aside for about 10 minutes or until gelatin has set.\\ 7. Meanwhile, to make the strawberries; hull and quarter the strawberries and toss in a bowl with the orange juice, vinegar and pepper.\end{tabular} &
\begin{tabular}[c]{@{}p{\linewidth}@{}}\textbf{Title: Ricotta Panna Cotta With Basil Balsamic Strawberries}\\ \textbf{ Ingredients:}\\ \textbf{ Ricotta Panna Cotta}\\ \textbf{ 2 1/2 teaspoons unflavored gelatin}\\ \textbf{ 5 tablespoons water}\\ \textbf{ 2 cups whipping cream}\\ \textbf{ 2/3 cup icing sugar}\\ \textbf{ 1 cup ricotta cheese}\\ \textbf{ 1/2 vanilla bean, slit lengthwise}\\ \textbf{ Basil Balsamic Strawberries}\\ \textbf{ 1 lb strawberry}\\ \textbf{ 1/3 cup orange juice}\\ \textbf{ 2 tablespoons balsamic vinegar}\\ \textbf{ 1/2 teaspoon cracked black pepper}\\ \textbf{ 6 large basil leaves, shredded}\\ \textbf{ Recipe:}\\ Panna Cotta: In a small bowl, soften the gelatin in cold water. Combine 1 cup of the cream, icing sugar and vanilla bean in a small pot. Bring to a boil and remove from the heat. Add the gelatin and stir to dissolve. Remove the vanilla bean and scrape the seeds into the cream.\\ Stir the remaining cream and ricotta. Pour into 8 5 - oz ramekins. Chill for at least 2 hours or up to overnight. Dip each ramekin into hot water, loosen with a knife and turn out onto individual plates.\\ Basil Balsamic Strawberries: Hull and cut the strawberries into quarters.\end{tabular} \\
\midrule
\multicolumn{2}{p{\linewidth}}{\small \textbf{Comment:} Note how {[}in the machine-generated recipe{]} the steps got misnumbered and how the gelatin never got cooked.}\\
\midrule
\begin{tabular}[c]{@{}p{\linewidth}@{}}\textbf{Title: Planet Hollywood Pot Stickers}\\ \textbf{ Ingredients:}\\ \textbf{ 1/4 lb. ground turkey}\\ \textbf{ 1/2 tsp. minced fresh ginger}\\ \textbf{ 1 tsp. minced green onion}\\ \textbf{ 1 tsp. minced water chestnuts}\\ \textbf{ 1/2 tsp. soy sauce}\\ \textbf{ 1/2 tsp. ground black pepper}\\ \textbf{ 1/4 tsp. crushed red pepper flakes (no seeds)}\\ \textbf{ 1/4 tsp. salt}\\ \textbf{ 1/8 tsp. garlic powder}\\ \textbf{ 1 egg, beaten}\\ \textbf{ Vegetable oil for frying}\\ \textbf{ 12 wonton wrappers (3 3-inch size)}\\ \textbf{ Hoisin sauce, on the side}\\ \textbf{ Recipe:}\\ Heat 2 Tbsp. oil in a large skillet over medium heat. Add ground turkey; sauté for 5 minutes, or until turkey is browned and crumbly. Stir in ginger, green onion, water chestnuts, soy sauce, black pepper, red pepper flakes, salt and garlic powder. Cook for an additional 2 minutes. Remove from heat; set aside.\\ Add 1 tsp. oil to a small skillet over medium heat. Add beaten egg; cook for 30 seconds, or until cooked. Remove from heat and cut egg into small pieces. Combine egg, turkey mixture, and 1 Tbsp. water in a small bowl.\end{tabular} & \begin{tabular}[c]{@{}p{\linewidth}@{}}\textbf{*Title: Planet Hollywood Pot Stickers}\\ \textbf{ Ingredients:}\\ \textbf{ 1/4 lb. ground turkey}\\ \textbf{ 1/2 tsp. minced fresh ginger}\\ \textbf{ 1 tsp. minced green onion}\\ \textbf{ 1 tsp. minced water chestnuts}\\ \textbf{ 1/2 tsp. soy sauce}\\ \textbf{ 1/2 tsp. ground black pepper}\\ \textbf{ 1/4 tsp. crushed red pepper flakes (no seeds)}\\ \textbf{ 1/4 tsp. salt}\\ \textbf{ 1/8 tsp. garlic powder}\\ \textbf{ 1 egg, beaten}\\ \textbf{ Vegetable oil for frying}\\ \textbf{ 12 wonton wrappers (3 3-inch size)}\\ \textbf{Hoisin sauce, on the side}\\ \textbf{ Recipe:}\\ In a small bowl, combine all the ingredients except the egg, wrappers and oil.\\ Add 1 tablespoon of the beaten egg.\\ Save the rest of the egg for later.\\ Preheat oil in a deep fryer or a deep saucepan to 375F.\\ Use enough oil to cover the pot stickers -- 1 to 2 inches should be enough.\\ Invert a small bowl or glass with a 3-inch diameter on the center of a wonton wrapper and cut around it to make a circle.\\ Repeat for the remaining wrappers.\\ Spoon 1/2 tablespoon of the turkey filling into the center of one wrapper.\end{tabular} \\
\midrule
\multicolumn{2}{p{\linewidth}}{\small \textbf{Comment:} Note the more complicated concepts {[}in the human-authored recipe{]}, like `all the ingredients except the egg, wrappers, and oil' and `save the rest of the egg for later.'} \\
\midrule
\begin{tabular}[c]{@{}p{\linewidth}@{}}\textbf{*Title: Corn And Lobster Chowder}\\ \textbf{ Ingredients:}\\ \textbf{ 1/4 lb thick slab bacon (rind removed)}\\ \textbf{ 1 tablespoon unsalted butter}\\ \textbf{ 2 cups diced onions (1/4-inch)}\\ \textbf{ 2 tablespoons all-purpose flour}\\ \textbf{ 4 cups chicken broth}\\ \textbf{ 2 bay leaves}\\ \textbf{ 1 teaspoon sweet paprika}\\ \textbf{ 2 russet potatoes, peeled and cut into 1/4-inch dice}\\ \textbf{ 3 sprigs fresh thyme}\\ \textbf{ 1 cup half-and-half}\\ \textbf{ 3 cups cooked fresh corn kernels}\\ \textbf{ 1 red bell peppers or 1 yellow bell pepper, cut into 1/4-inch dice}\\ \textbf{ 4 scallions, very thinly sliced}\\ \textbf{ salt and black pepper, to taste}\\ \textbf{ 2 cups cooked lobsters, cut into 1/2-inch dice (fresh or frozen)}\\ \textbf{ 1/4 cup flat leaf parsley}\\ \textbf{ Recipe:}\\ Cook bacon in a 3-quart saucepan over medium heat until crisp, about 8 minutes. Remove to paper towel to drain.\\ Add butter and onion to the drippings in the pan and cook over medium heat until onion is clear, about 5 minutes. Add the flour and cook, stirring constantly, for 2 minutes.\\ Add broth, bay leaves, paprika, potatoes, and thyme. Bring to a boil, reduce to a simmer, and cook for 10 minutes, stirring occasionally.\\ Add the corn, peppers, scallions, salt and pepper. Bring back to a boil, reduce heat to a simmer, and cook for 5 minutes.\end{tabular} & \begin{tabular}[c]{@{}p{\linewidth}@{}}\textbf{Title: Corn And Lobster Chowder}\\ \textbf{ Ingredients:}\\ \textbf{ 1/4 lb thick slab bacon (rind removed)}\\ \textbf{ 1 tablespoon unsalted butter}\\ \textbf{ 2 cups diced onions (1/4-inch)}\\ \textbf{ 2 tablespoons all-purpose flour}\\ \textbf{ 4 cups chicken broth}\\ \textbf{ 2 bay leaves}\\ \textbf{ 1 teaspoon sweet paprika}\\ \textbf{ 2 russet potatoes, peeled and cut into 1/4-inch dice}\\ \textbf{ 3 sprigs fresh thyme}\\ \textbf{ 1 cup half-and-half}\\ \textbf{ 3 cups cooked fresh corn kernels}\\ \textbf{ 1 red bell peppers or 1 yellow bell pepper, cut into 1/4-inch dice}\\ \textbf{ 4 scallions, very thinly sliced}\\ \textbf{ salt and black pepper, to taste}\\ \textbf{ 2 cups cooked lobsters, cut into 1/2-inch dice (fresh or frozen)}\\ \textbf{ 1/4 cup flat leaf parsley}\\ \textbf{ Recipe:}\\ Cut bacon into small dice and place in a large pot over low heat.\\ Cook, stirring, to render the fat, 5 to 7 minutes.\\ Add butter and let it melt.\\ Add onion and cook over low heat, stirring occasionally, until wilted, about 10 minutes.\\ Add flour; cook, stirring, for 1 minute longer.\\ Simmer broth, bay leaves, and paprika in the pot for 5 minutes to flavor broth.\\ Add potatoes and thyme; cook until potatoes are just tender, about 15 minutes.\\ Add half-and-half, corn, peppers, and scallions; cook 10 minutes.\\ Season with the salt and pepper.\\ Add lobster and parsley just before serving hot.\end{tabular} \\
\midrule
\multicolumn{2}{p{\linewidth}}{\small \textbf{Comment:} Note how the bacon drippings are supposed to be drained out on a paper towel but then are used in the next step, and note how the soup is supposed to be boiled and then re-boiled.} \\
\bottomrule
\end{tabular}
\caption{The training materials used in the recipe domain for the Comparison trainings. The passages marked with * were shown in the Example training, along with the comments with the bracketed text removed.}
\label{tab:recipe_training}
\end{table*}
